# Supplementary material for: A new method to correct for host star variability in multi-epoch observations of exoplanet transmission spectra
Source: arXiv:2207.01606 ancillary file (2022-07-04)
Supplement: Supplementary file 1 [file GMOS_WASP-19b_supplementary_comp.pdf]

Table 1: Best fit GP hyperparameters and their uncertainties for the white transit light curve fits. Similar to Table 4. in the paper, the column 'No.' specifies the transit observation, 'Method' specifies the method used to fit the white transit light curves, and 'GP regressors' specifies the GP regressor combination used. 'A' is the amplitude hyperparameter, and $\eta_t$, $\eta_c$, $\eta_a$ are the time, comparison star white light curve length scale hyperparameters respectively.

| No. | Method | GP regressors | ln(A) | ln($\eta_t$) | ln($\eta_c$) | ln($\eta_a$) | $\sigma_w$ [ppm] |
|---|---|---|---|---|---|---|---|
| 1 | New | Time, Comp | $-4.67^{+2.82}_{-1.76}$ | $24.22^{+2.51}_{-1.68}$ | $-1.06^{+1.94}_{-1.27}$ | – | $383^{+35}_{-28}$ |
| | Conventional | Airmass | $-14.02^{+0.74}_{-0.44}$ | – | – | $-8.17^{+0.92}_{-0.68}$ | $395^{+39}_{-30}$ |
| 2 | New | Time, Comp | $-4.77^{+3.11}_{-2.74}$ | $24.1^{+2.99}_{-3.04}$ | $2.23^{+2.45}_{-2.32}$ | – | $373^{+25}_{-25}$ |
| | Conventional | Airmass | $-11.82^{+2.11}_{-1.22}$ | $-3.55^{+2.08}_{-1.59}$ | – | – | $431^{+27}_{-23}$ |
| 3 | New | Time, Comp | $-4.53^{+2.64}_{-1.99}$ | – | $24.37^{+1.97}_{-1.66}$ | – | $345^{+24}_{-21}$ |
| | Conventional | Time | $-12.77^{+1.22}_{-0.81}$ | $-5.81^{+1.07}_{-0.84}$ | – | – | $338^{+24}_{-22}$ |
| 4 | New | Time, Comp, Airmass | $-6.19^{+3.31}_{-2.39}$ | $23.3^{+3.16}_{-2.44}$ | $430.8^{+363.91}_{-308.02}$ | $-0.9^{+2.38}_{-1.71}$ | $353^{+25}_{-23}$ |
| | Conventional | Time | $-13.82^{+0.88}_{-0.65}$ | $-7.64^{+1.06}_{-0.89}$ | – | – | $375^{+25}_{-25}$ |
| 5 | New | Time, Comp | $-5.96^{+3.28}_{-2.3}$ | $23.51^{+3.09}_{-2.3}$ | $-1.9^{+2.19}_{-1.58}$ | – | $326^{+24}_{-22}$ |
| | Conventional | Time, Airmass | $-14.23^{+1.07}_{-0.71}$ | $-8.29^{+1.16}_{-0.94}$ | – | $484.2^{+317.75}_{-319.56}$ | $380^{+28}_{-26}$ |
| 6 | New | Comp | $-3.34^{+3.03}_{-2.32}$ | – | $25.53^{+2.45}_{-1.99}$ | – | $402^{+30}_{-25}$ |
| | Conventional | Time | $-14.21^{+1.33}_{-0.87}$ | $-5.57^{+1.87}_{-1.22}$ | – | – | $399^{+30}_{-25}$ |
| 7 | New | Time, Comp | $-3.61^{+2.65}_{-1.94}$ | $25.62^{+2.44}_{-1.79}$ | $0.26^{+2.61}_{-1.52}$ | – | $378^{+39}_{-31}$ |
| | Conventional | Time, Airmass | $-13.82^{+0.89}_{-0.62}$ | $123.54^{+364.52}_{-129.31}$ | $-4.38^{+59.95}_{-1.05}$ | – | $402^{+42}_{-36}$ |
| 8 | New | Time, Comp | $-4.85^{+2.6}_{-1.11}$ | $26.512^{+2.34}_{-1.08}$ | $-0.38^{+1.6}_{-1.25}$ | – | $753^{+65}_{-58}$ |
| | Conventional | Time | $-12.48^{+0.73}_{-0.42}$ | $-8.08^{+1.09}_{-0.61}$ | – | – | $1051.0^{+91}_{-81}$ |

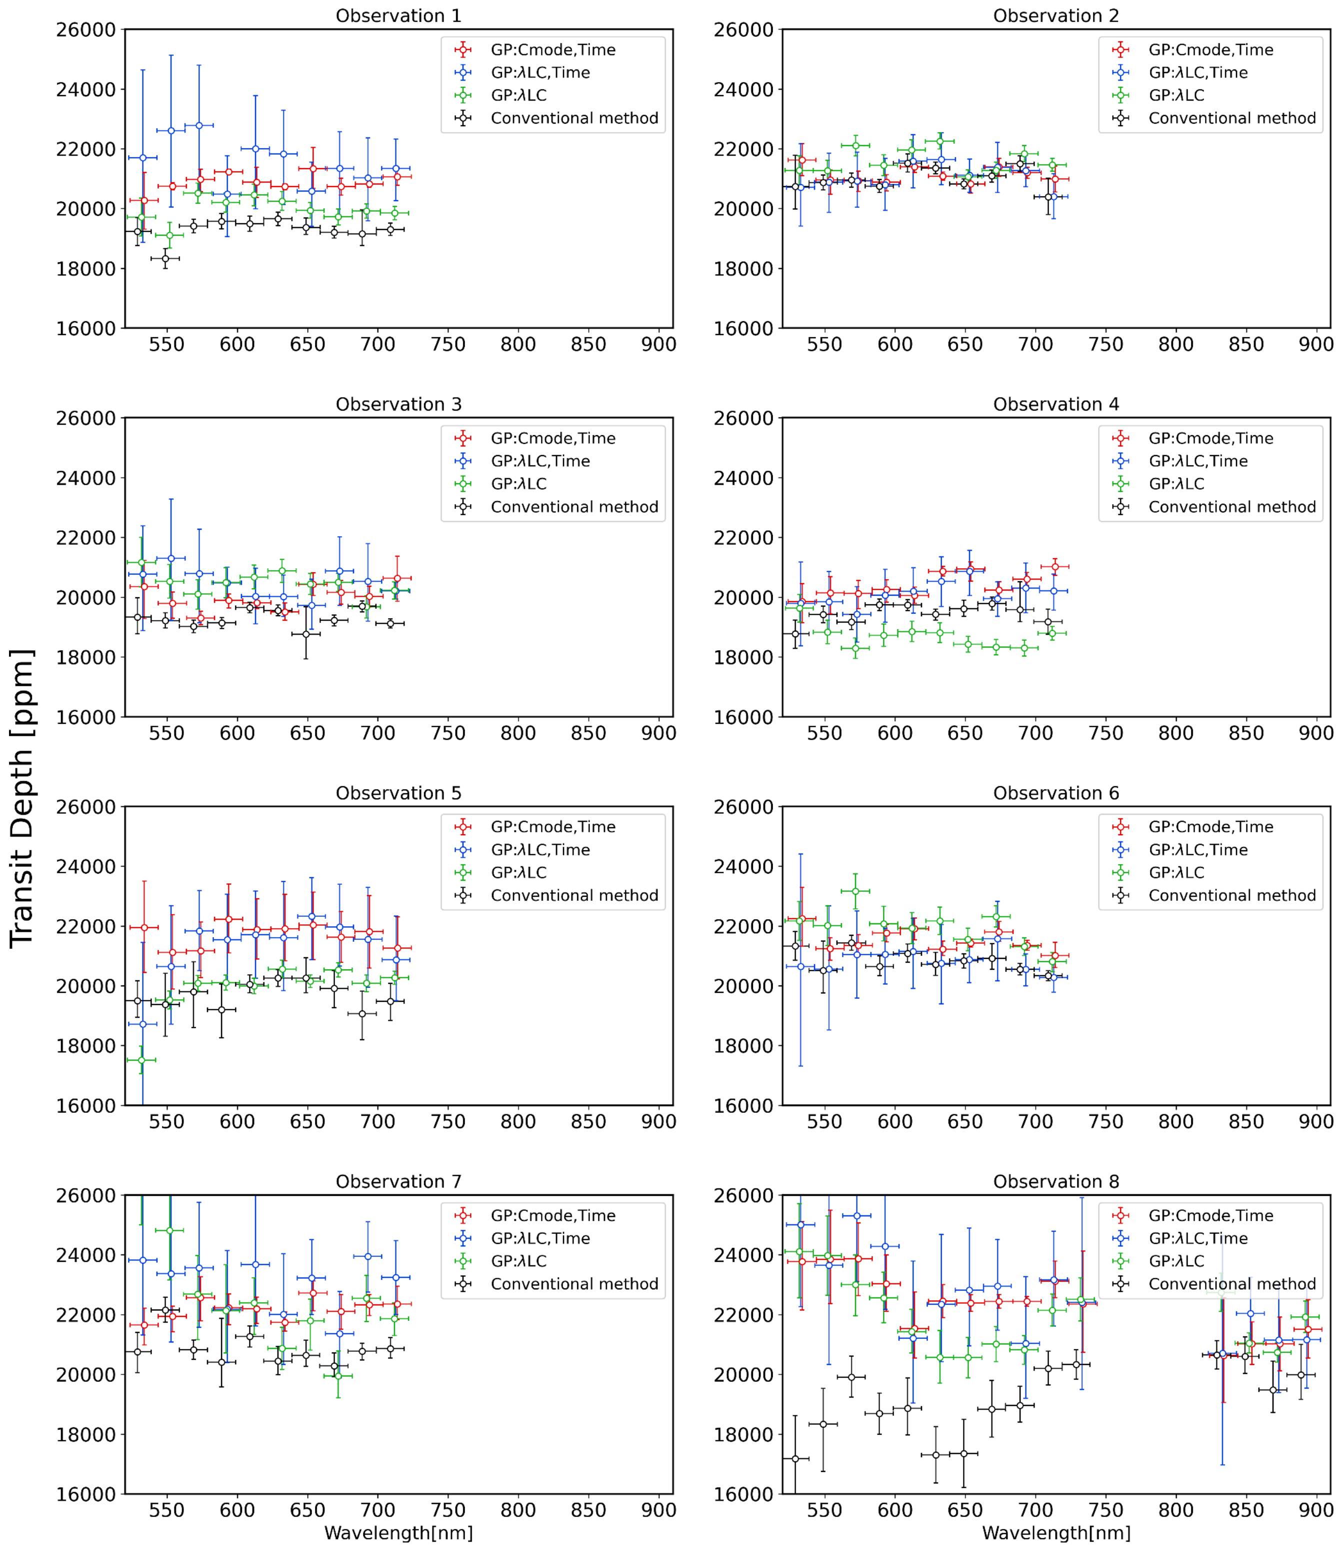


Figure 1: GMOS R150 transmission spectrum for each of the eight transits obtained using different methods to fit the spectroscopic light curves. The red, blue and green points are obtained by fitting the target spectroscopic light curves ($\lambda$LC) using the following GP regressor combinations respectively: common-mode and time, comparison $\lambda$LC and time, and comparison $\lambda$LC. The black points show the transmission spectrum obtained from the conventional method of fitting the target divided by the comparison star $\lambda$LC.

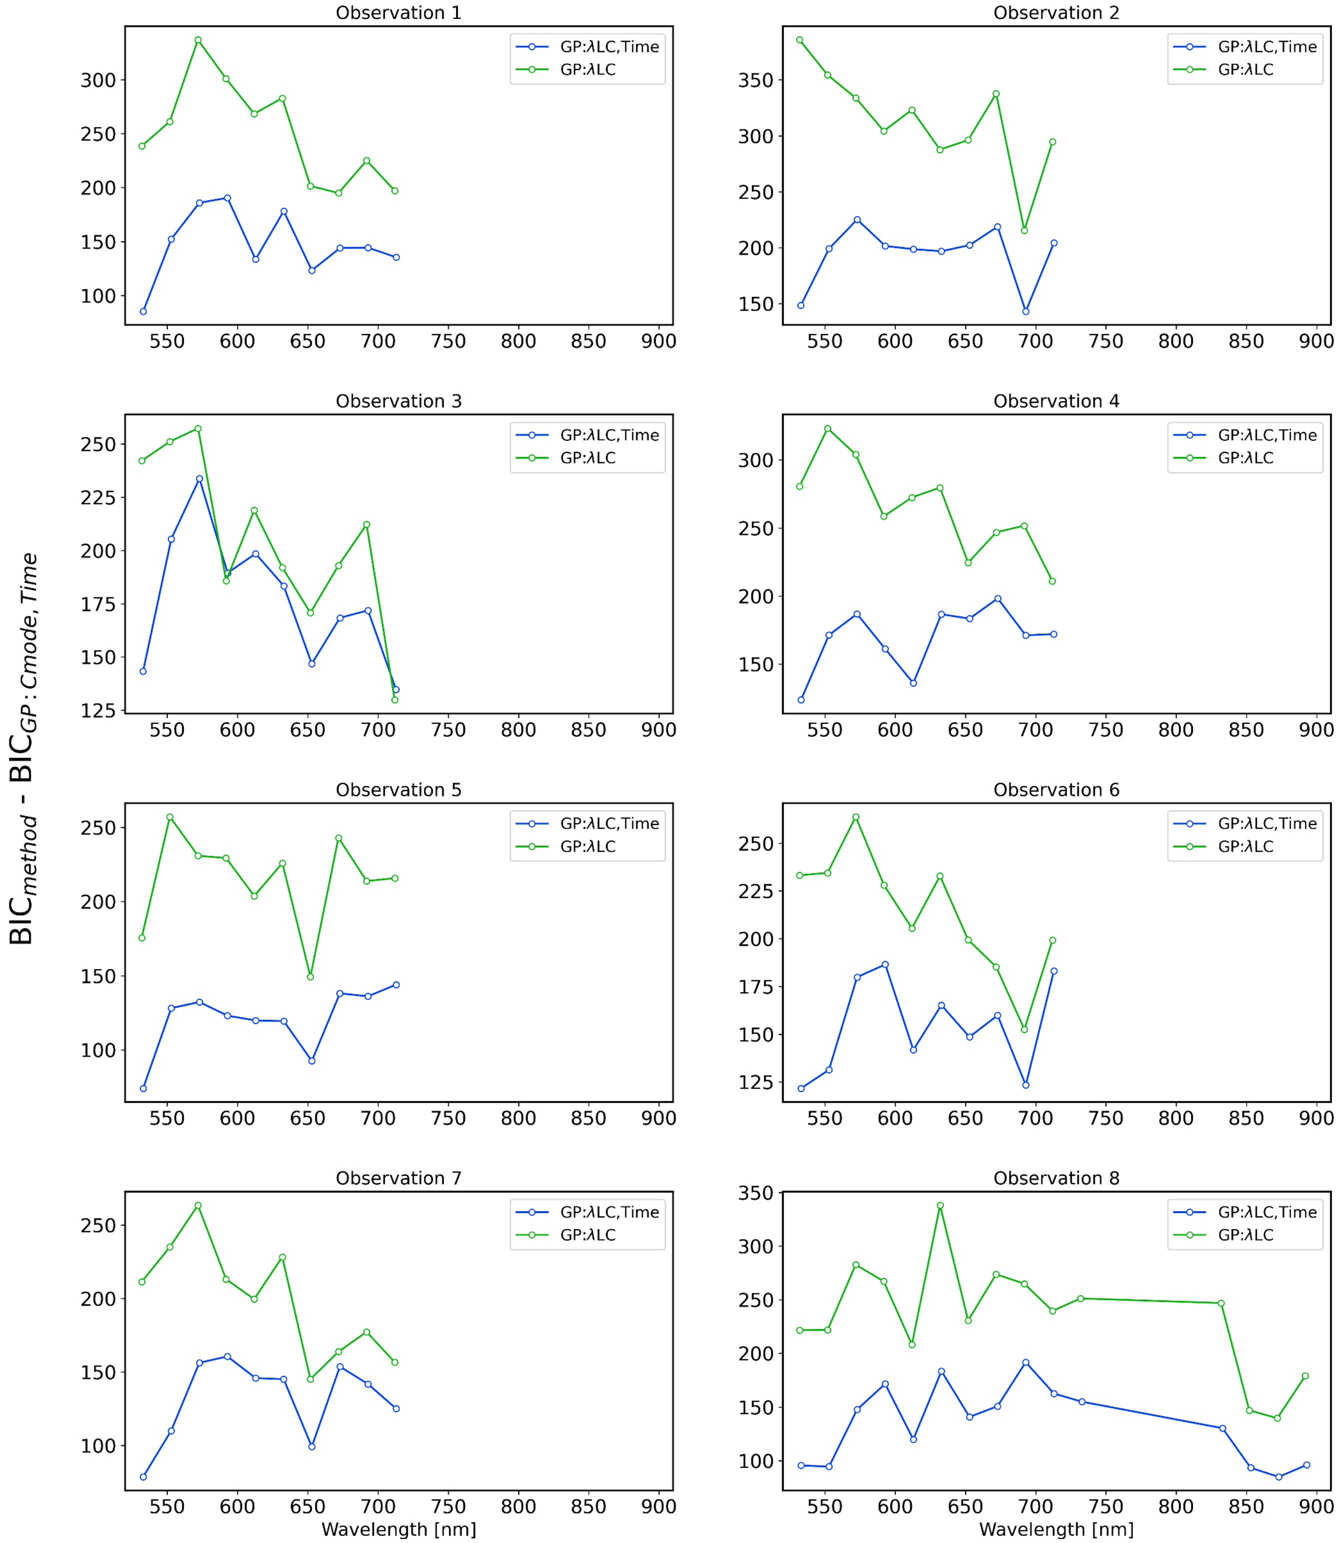


Figure 2: BIC comparison for each wavelength bin for the spectroscopic light curve fits corresponding to the transmission spectra obtained using the various GP regressor combinations of the new method as shown in Figure 1. The blue points show the $\Delta BIC$ for the comparison$\lambda$LC and time combination with respect to common-mode and time combination. The green points show the $\Delta BIC$ for comparison $\lambda$LC with respect to the common-mode and time combination. We find that the common-mode and time combination is the best combination with the lowest BIC among all methods. When using the comparison $\lambda$LC as one of the GP regressors, using time as well as an additional regressor (blue points here) gives a better fit in terms of the BIC as seen in this figure.

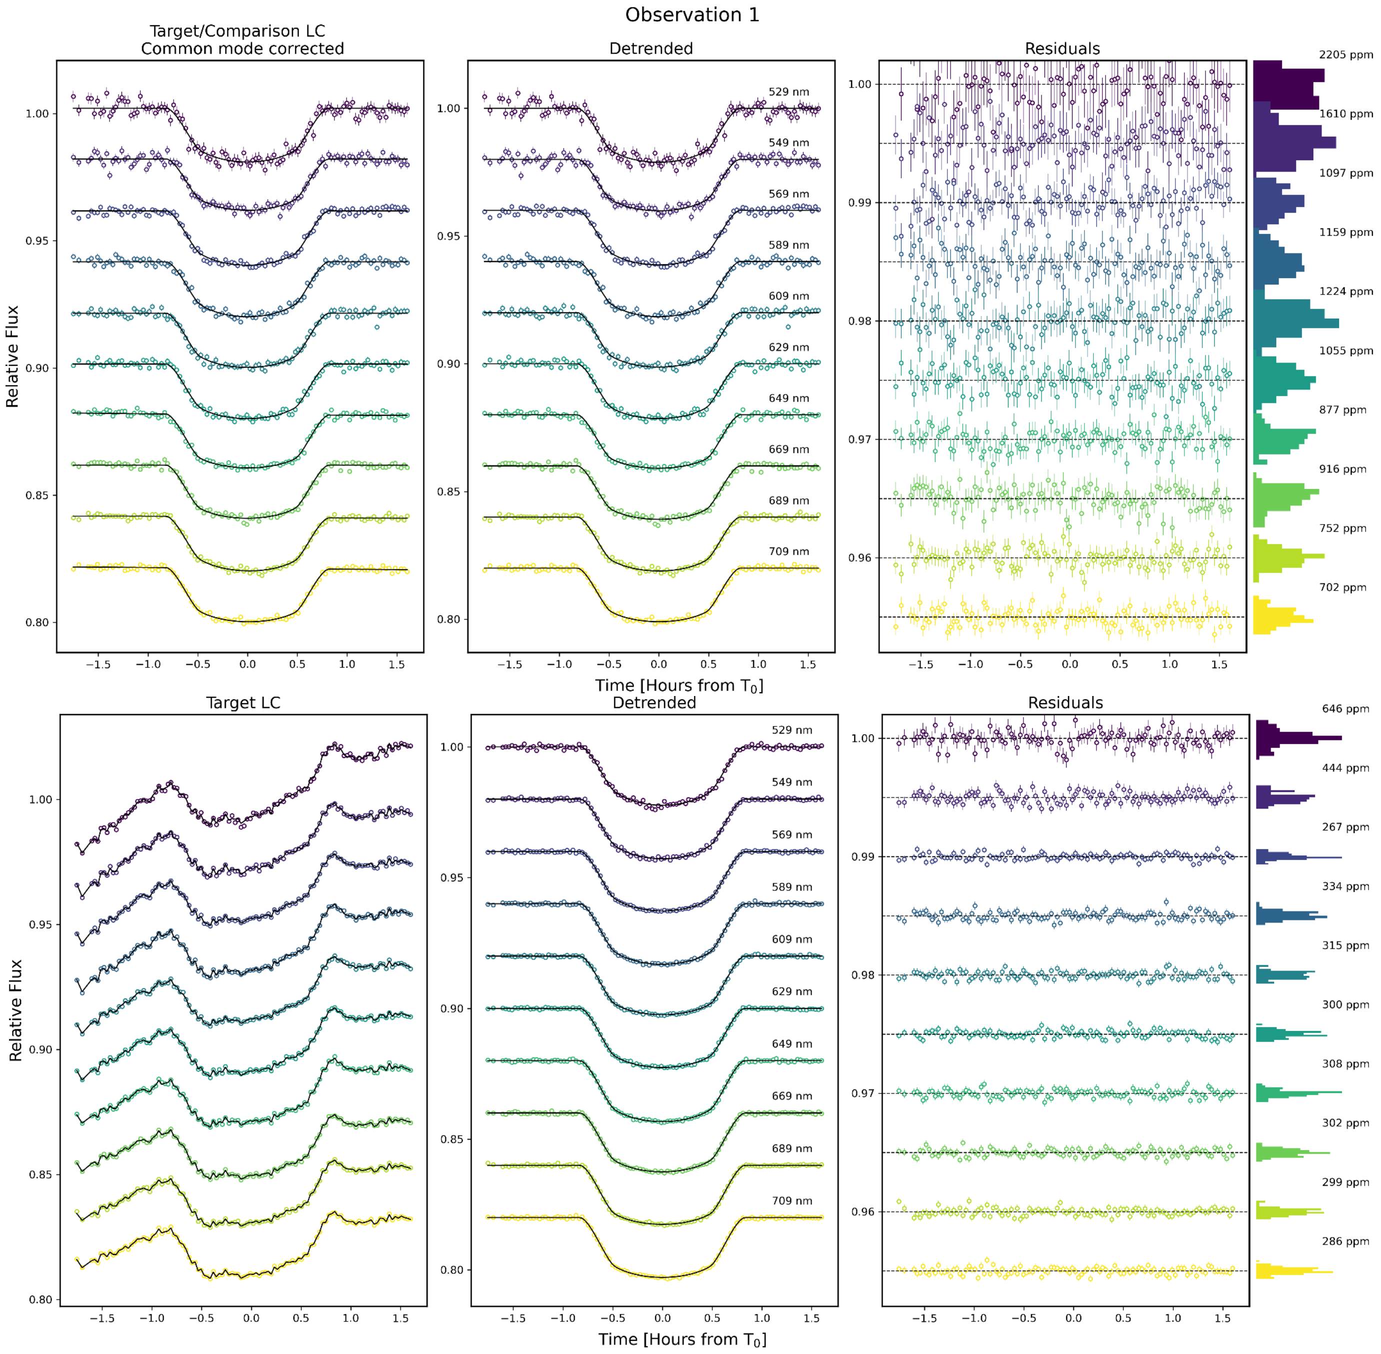


Figure 3: Spectroscopic light curves for observation 1 fit using the conventional method (top three panels) of fitting the common-mode corrected Target/Comparison $\lambda$LC as described in Section 5.3.1, and the new method (bottom three panels) of fitting the Target $\lambda$LCs using the common-mode trend as a GP regressor as described in Section 5.3.2. The leftmost panel for each method shows the best fit to the light curves for each wavelength bin, the middle panel shows the detrended light curves with their best fit transit models, and the rightmost panel shows the corresponding residuals, their histograms, and RMS of the residuals.

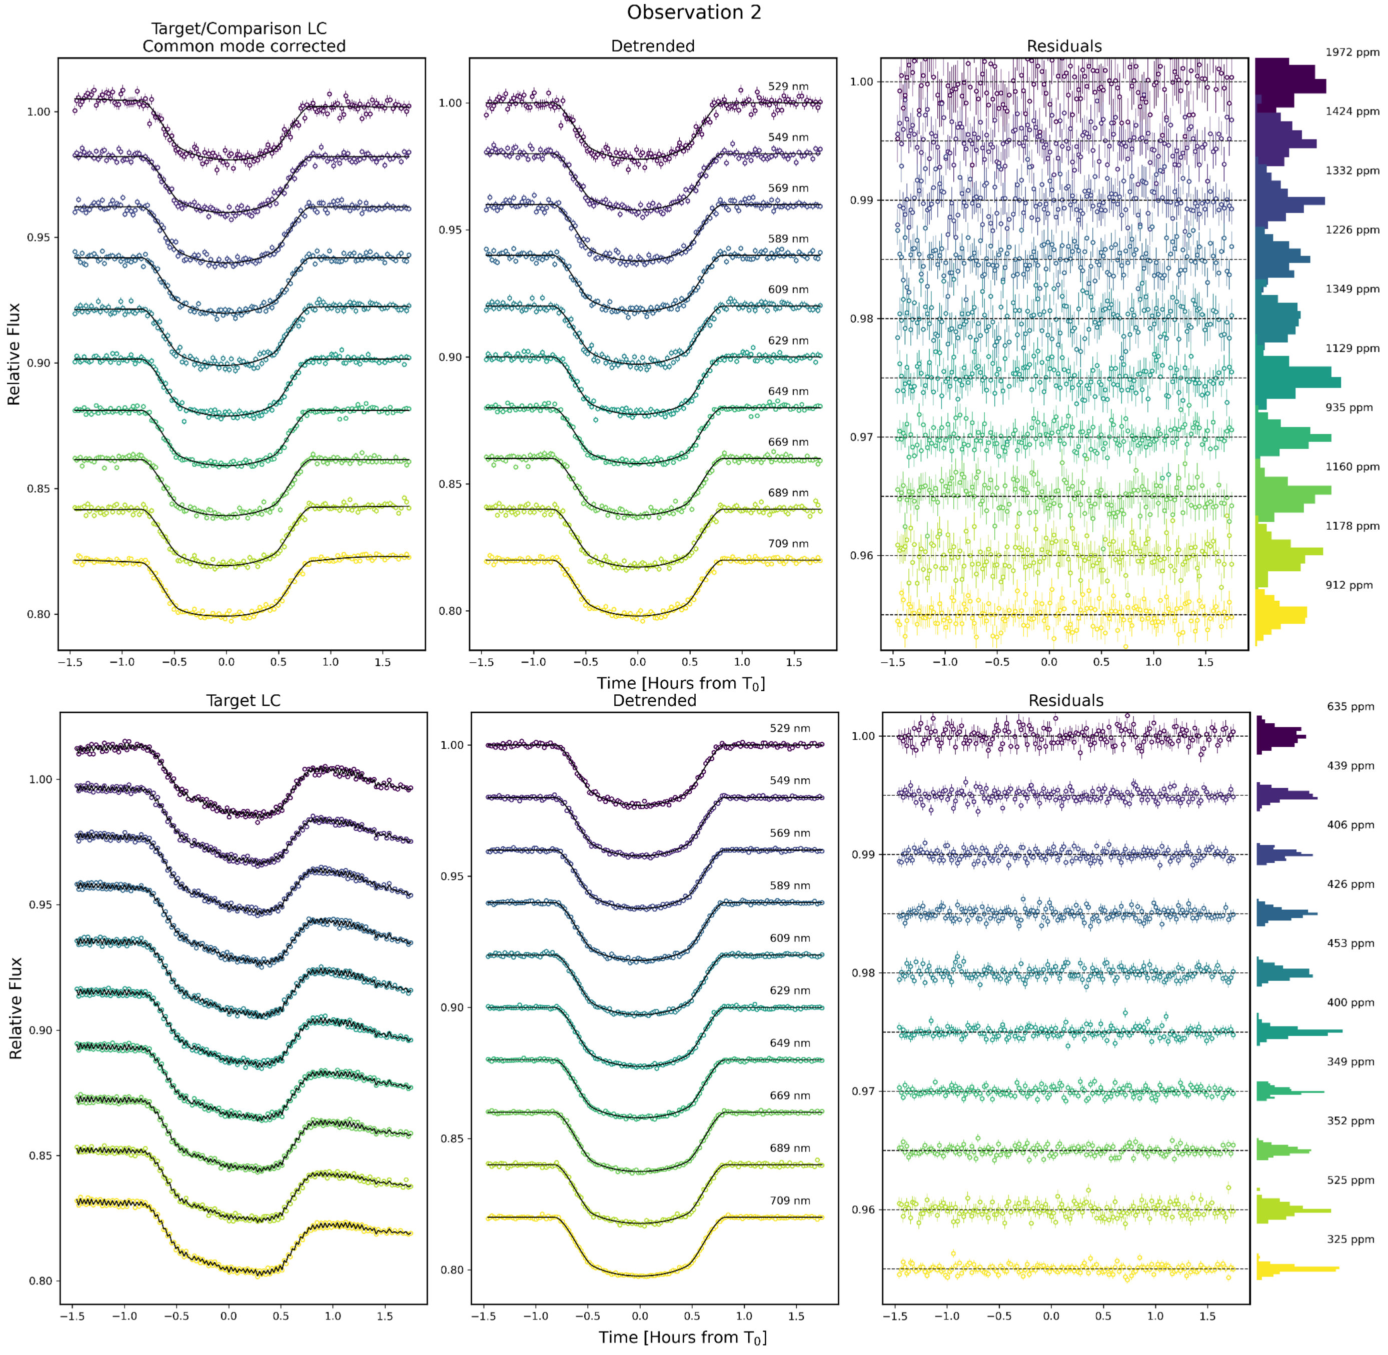


Figure 4: Same as Figure 3 for observation 2.

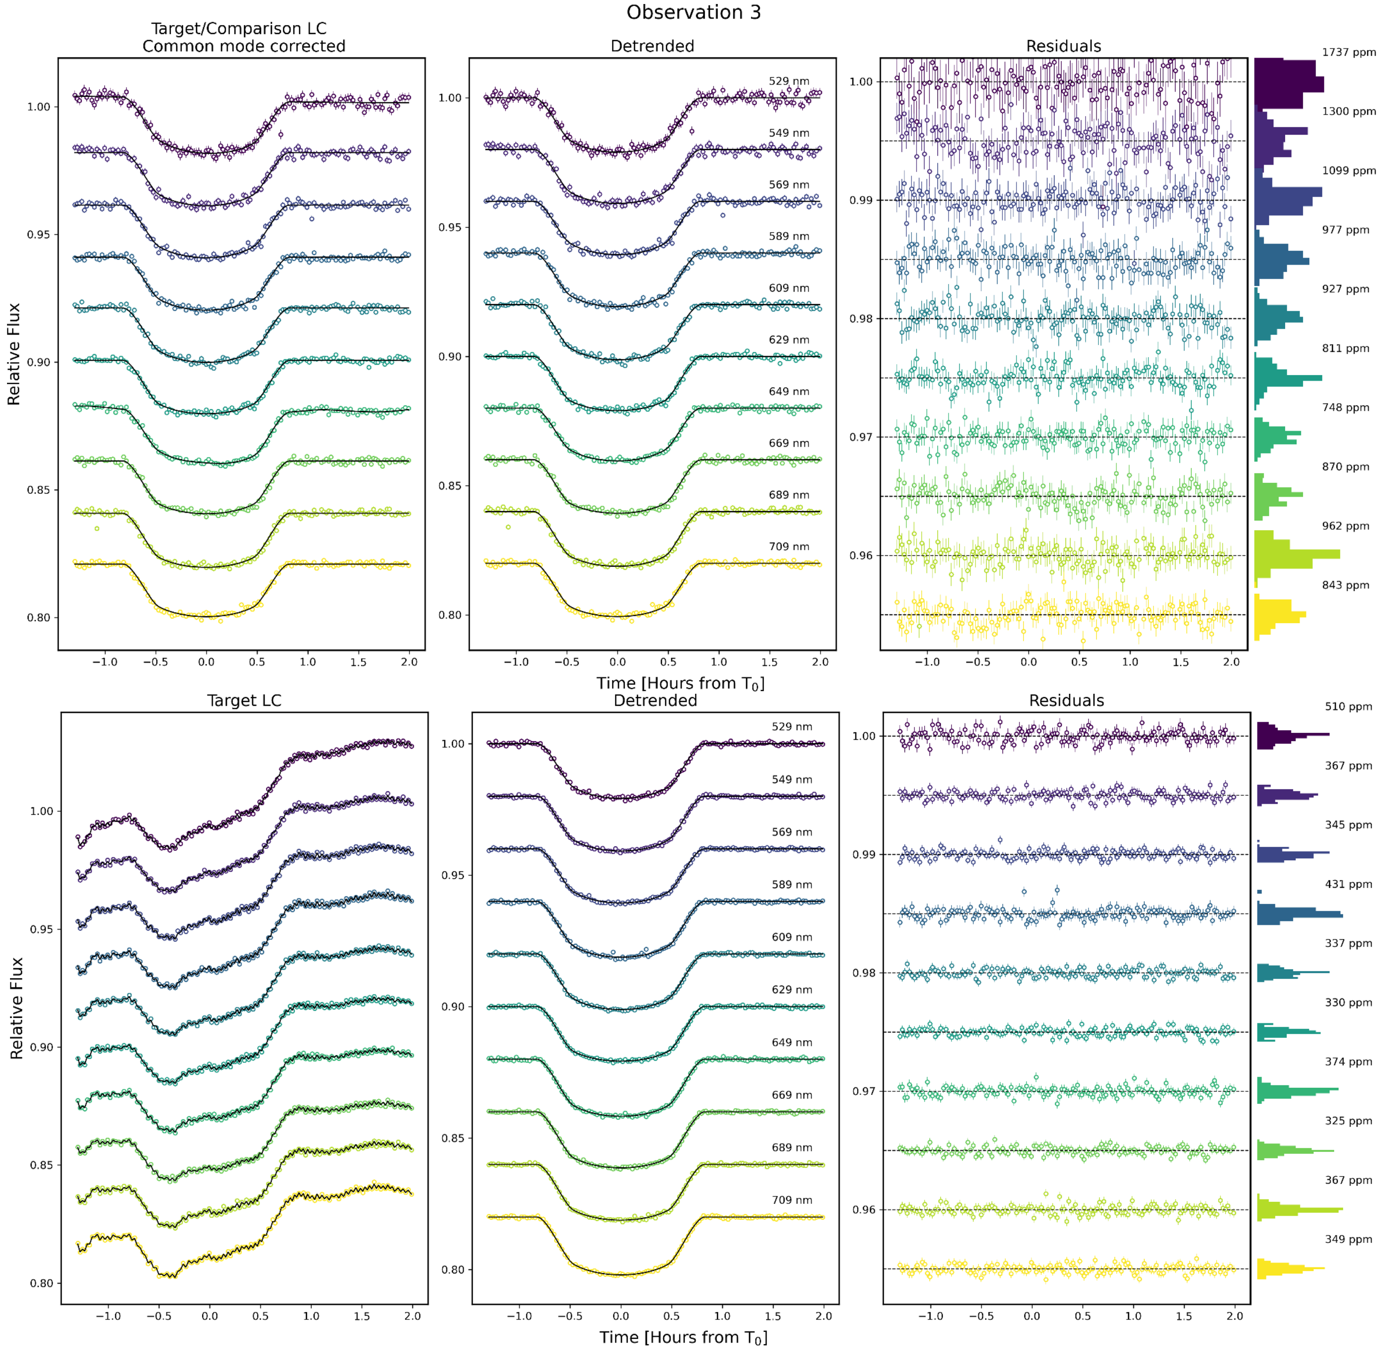


Figure 5: Same as Figure 3 for observation 3.

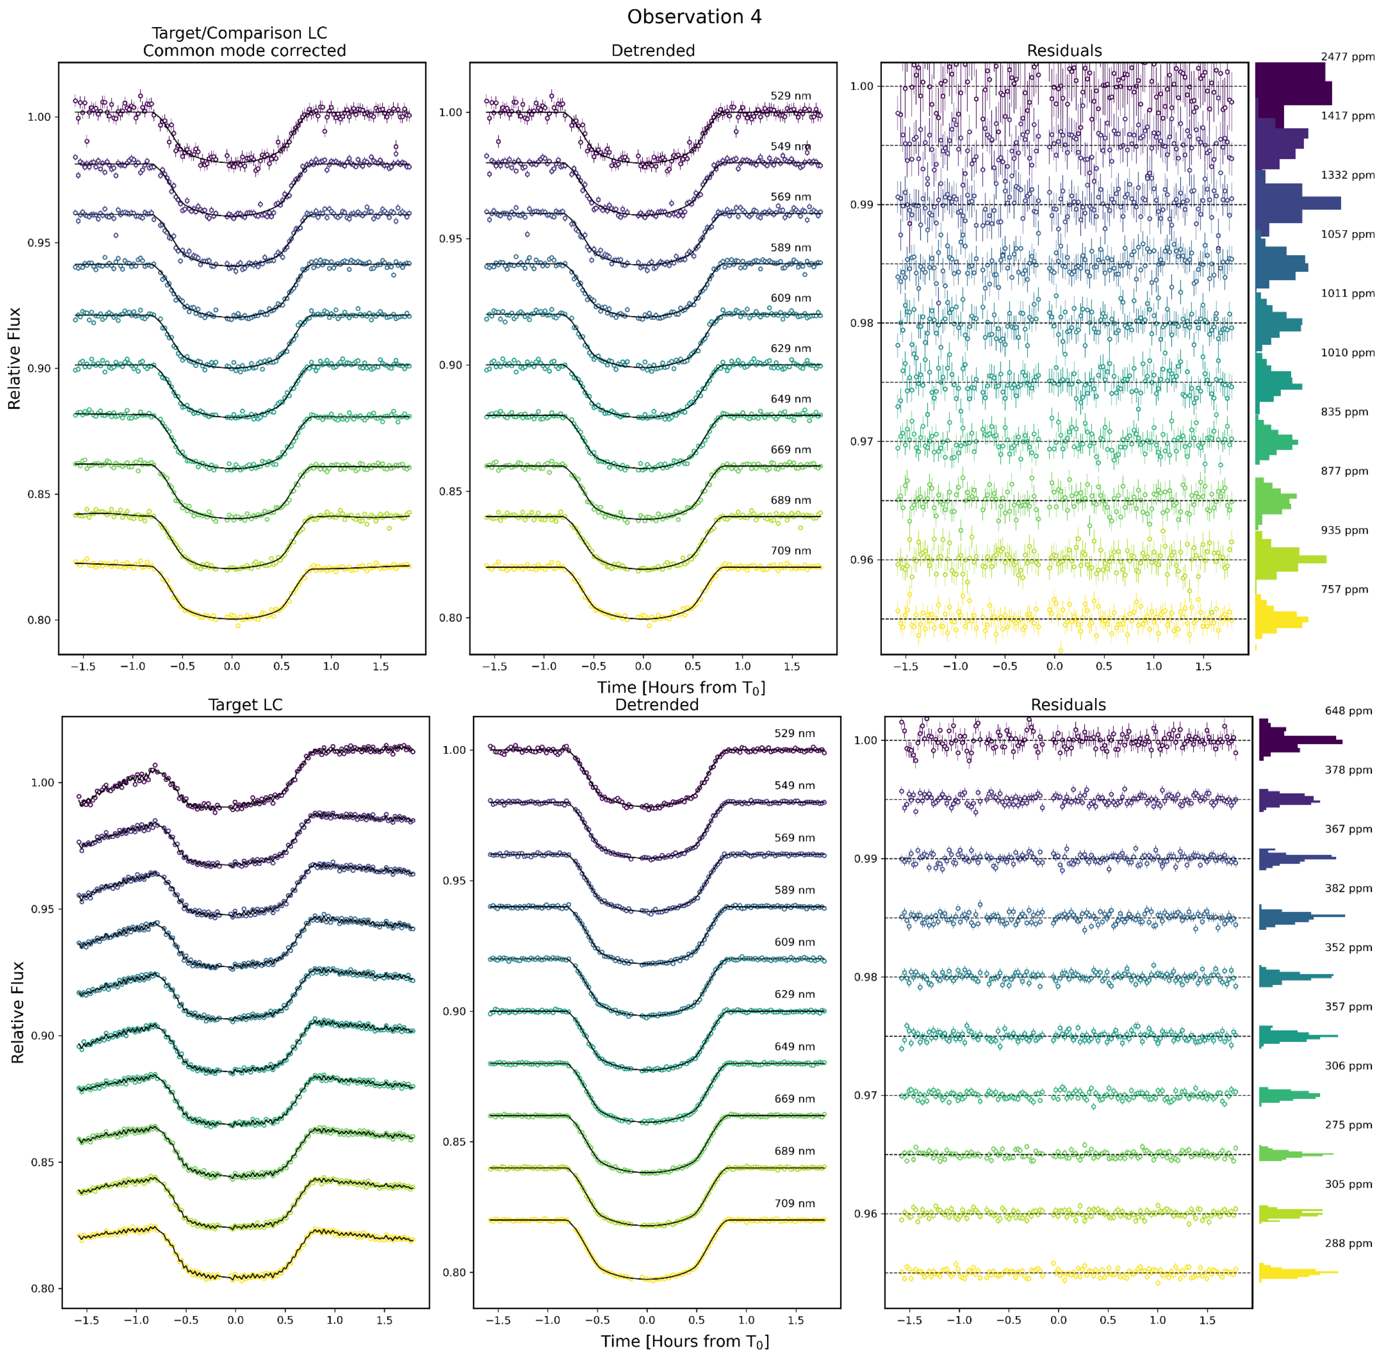


Figure 6: Same as Figure 3 for observation 4.

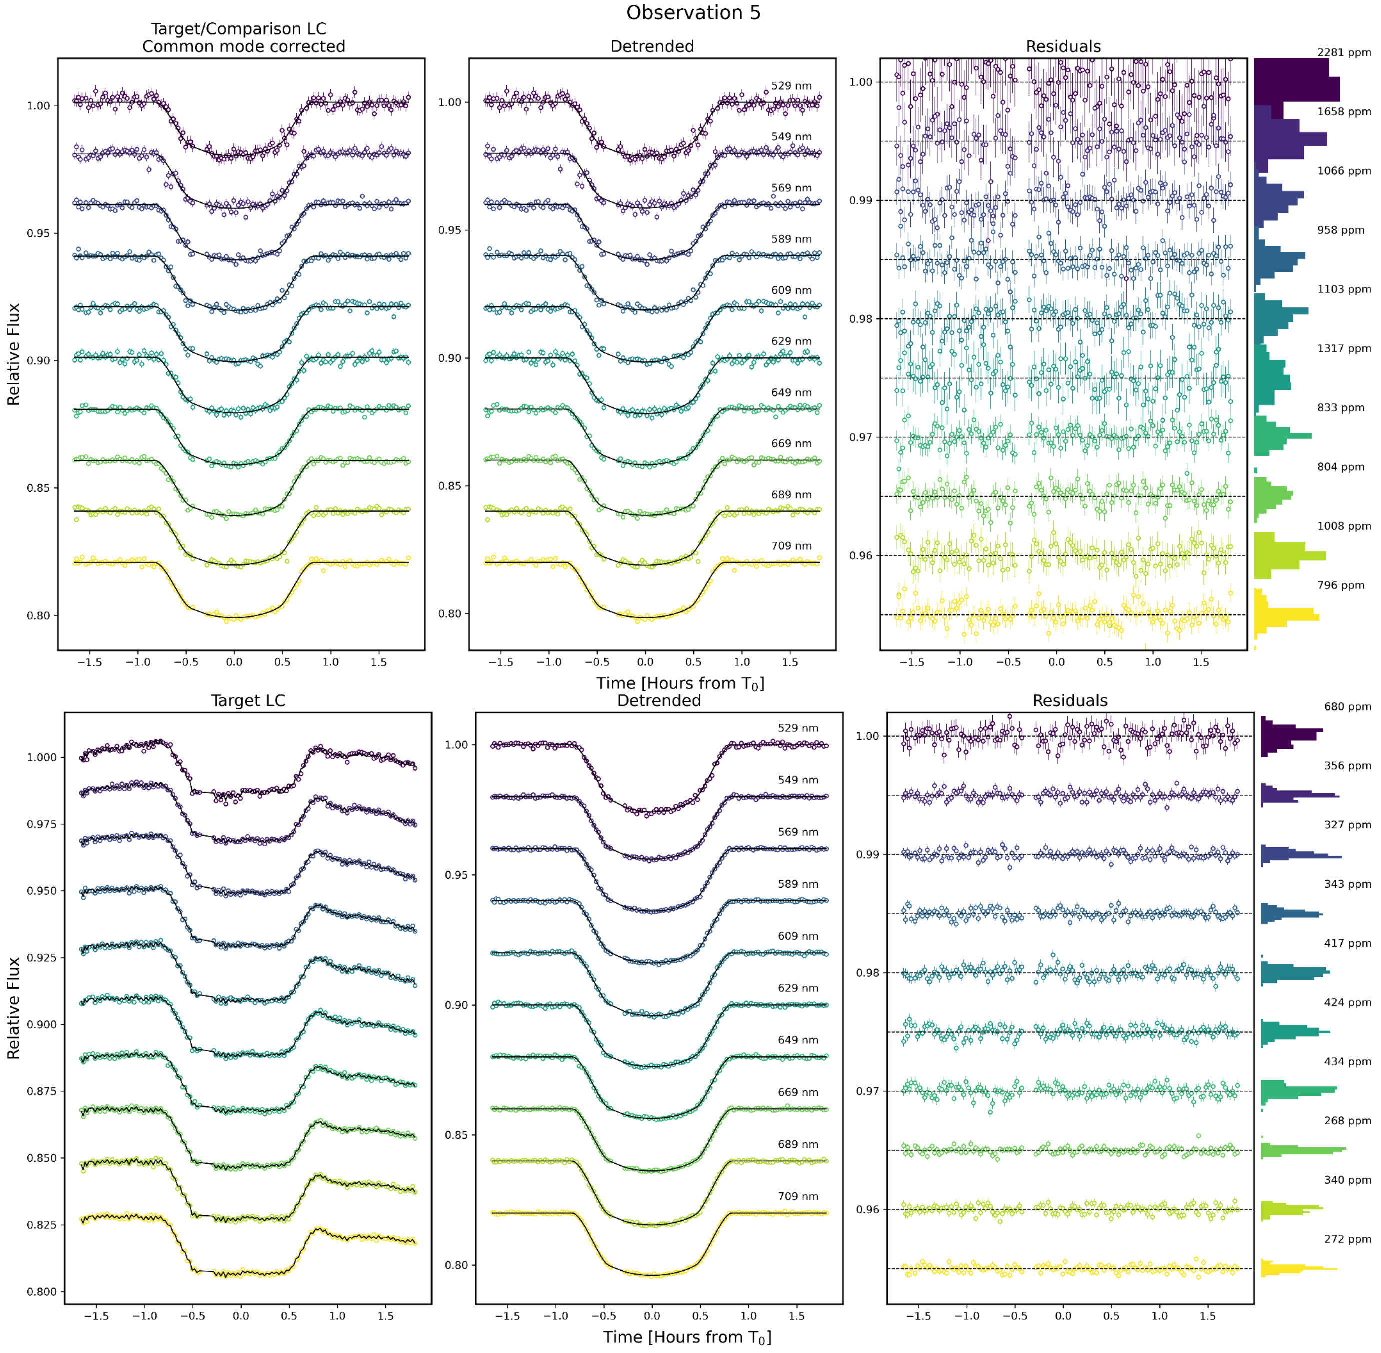


Figure 7: Same as Figure 3 for observation 5.

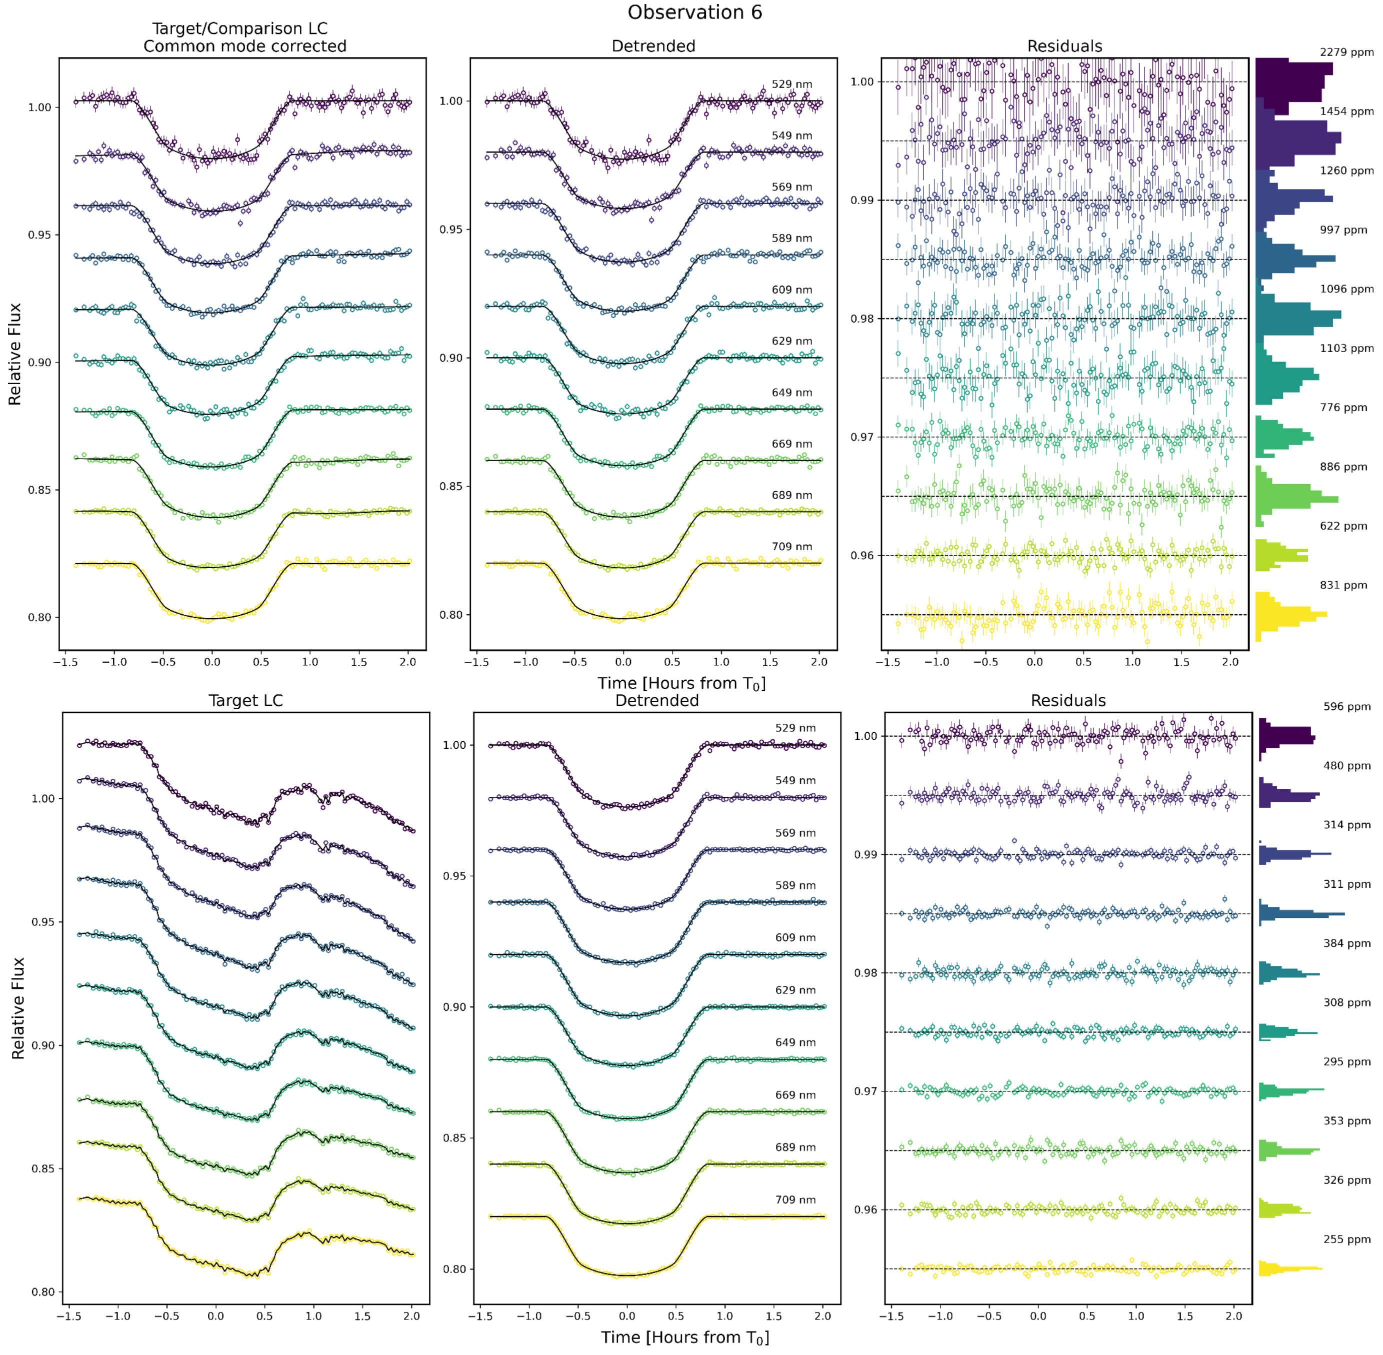


Figure 8: Same as Figure 3 for observation 6.

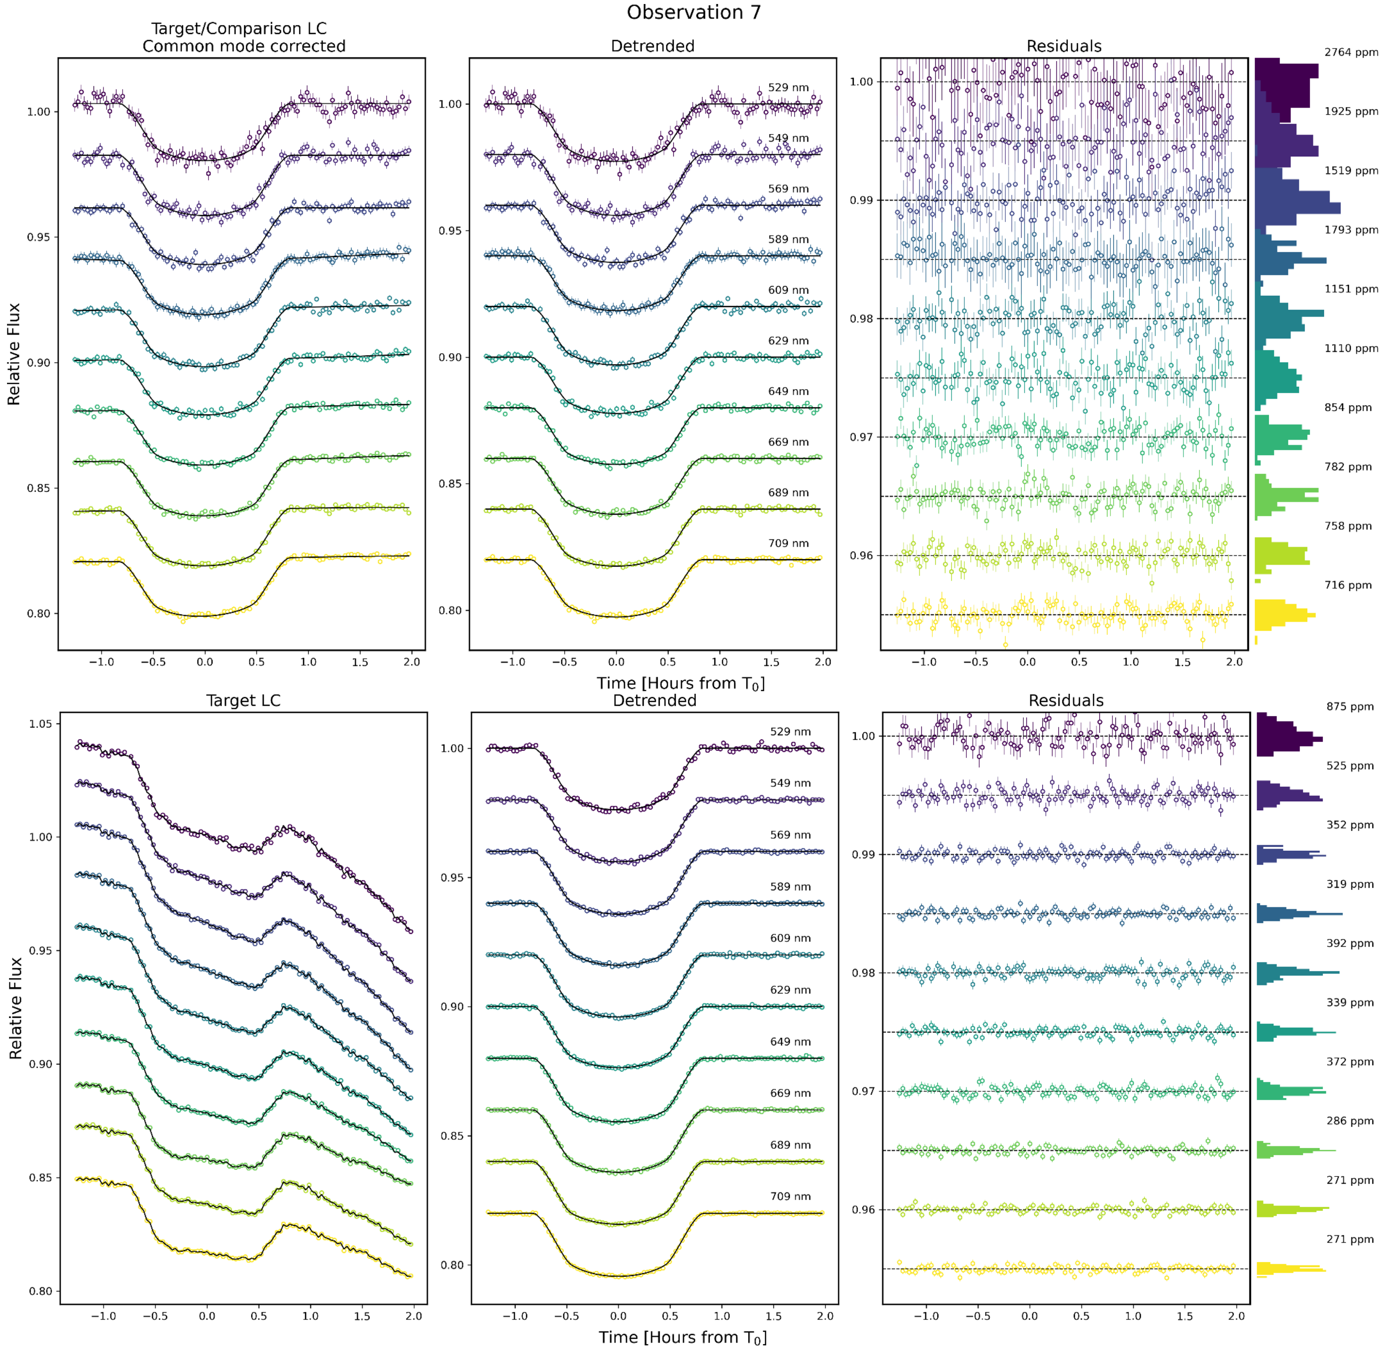


Figure 9: Same as Figure 3 for observation 7.

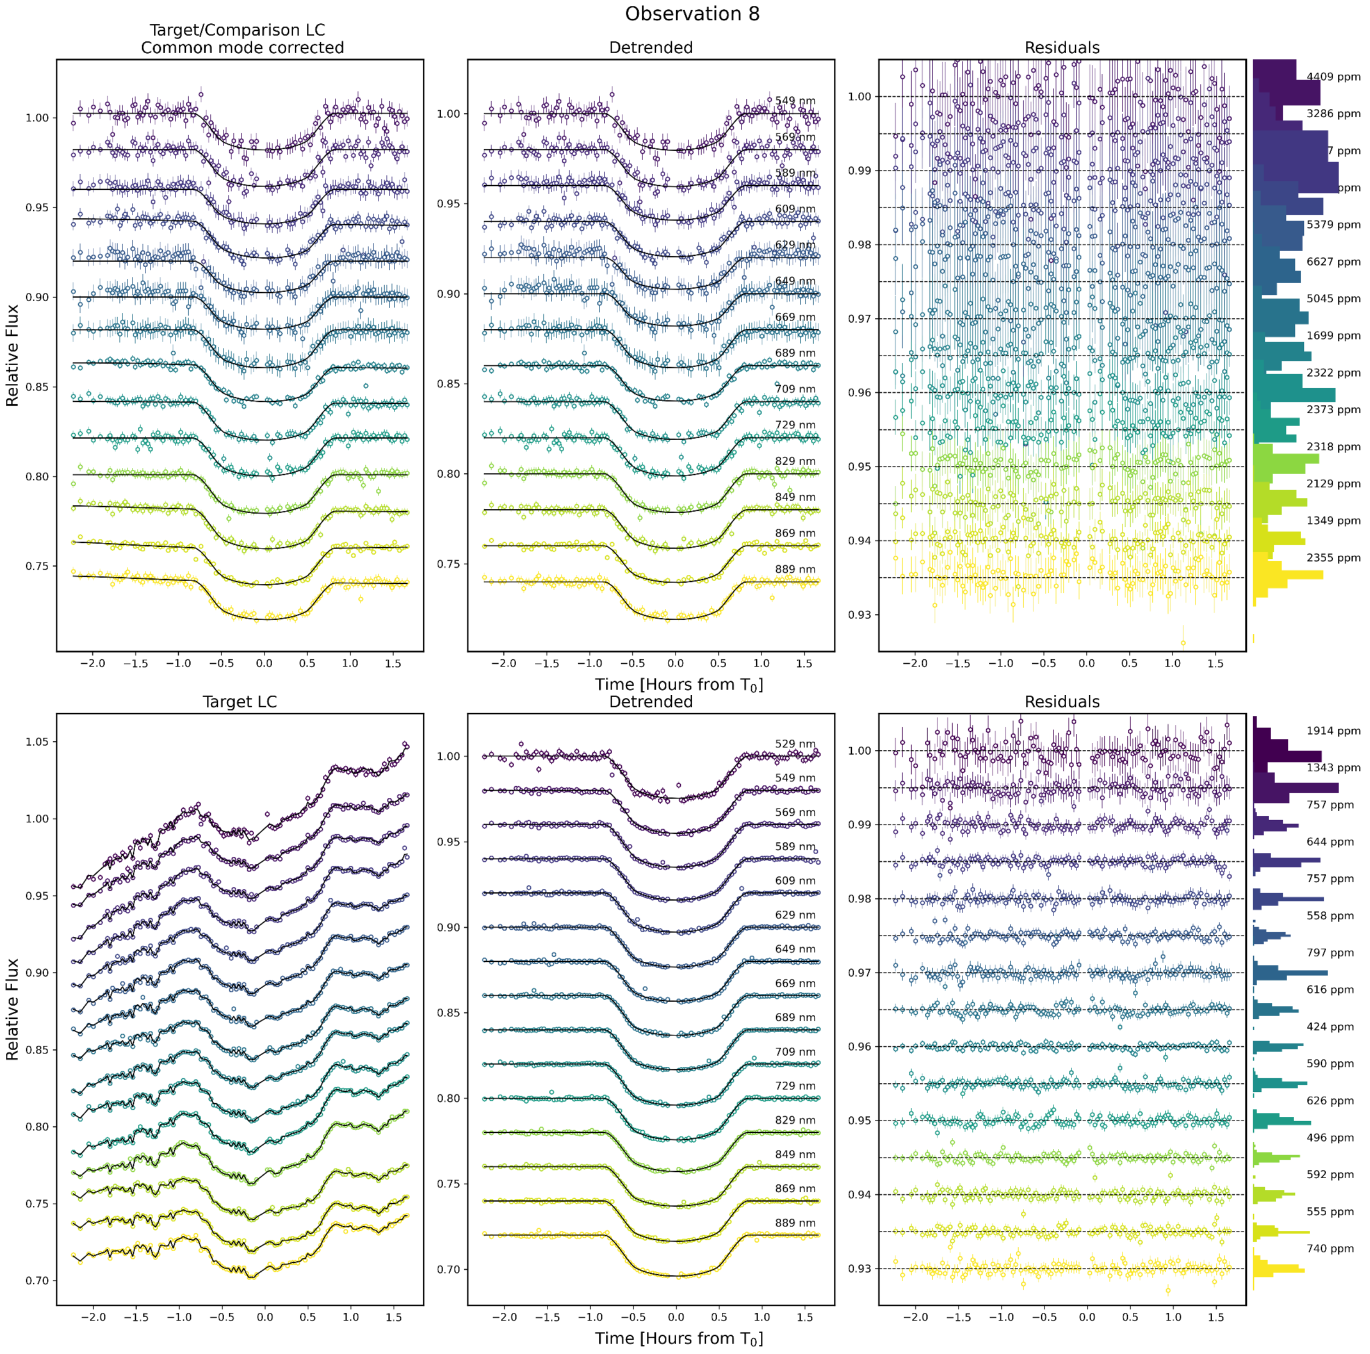


Figure 10: Same as Figure 3 for observation 8 (R150).

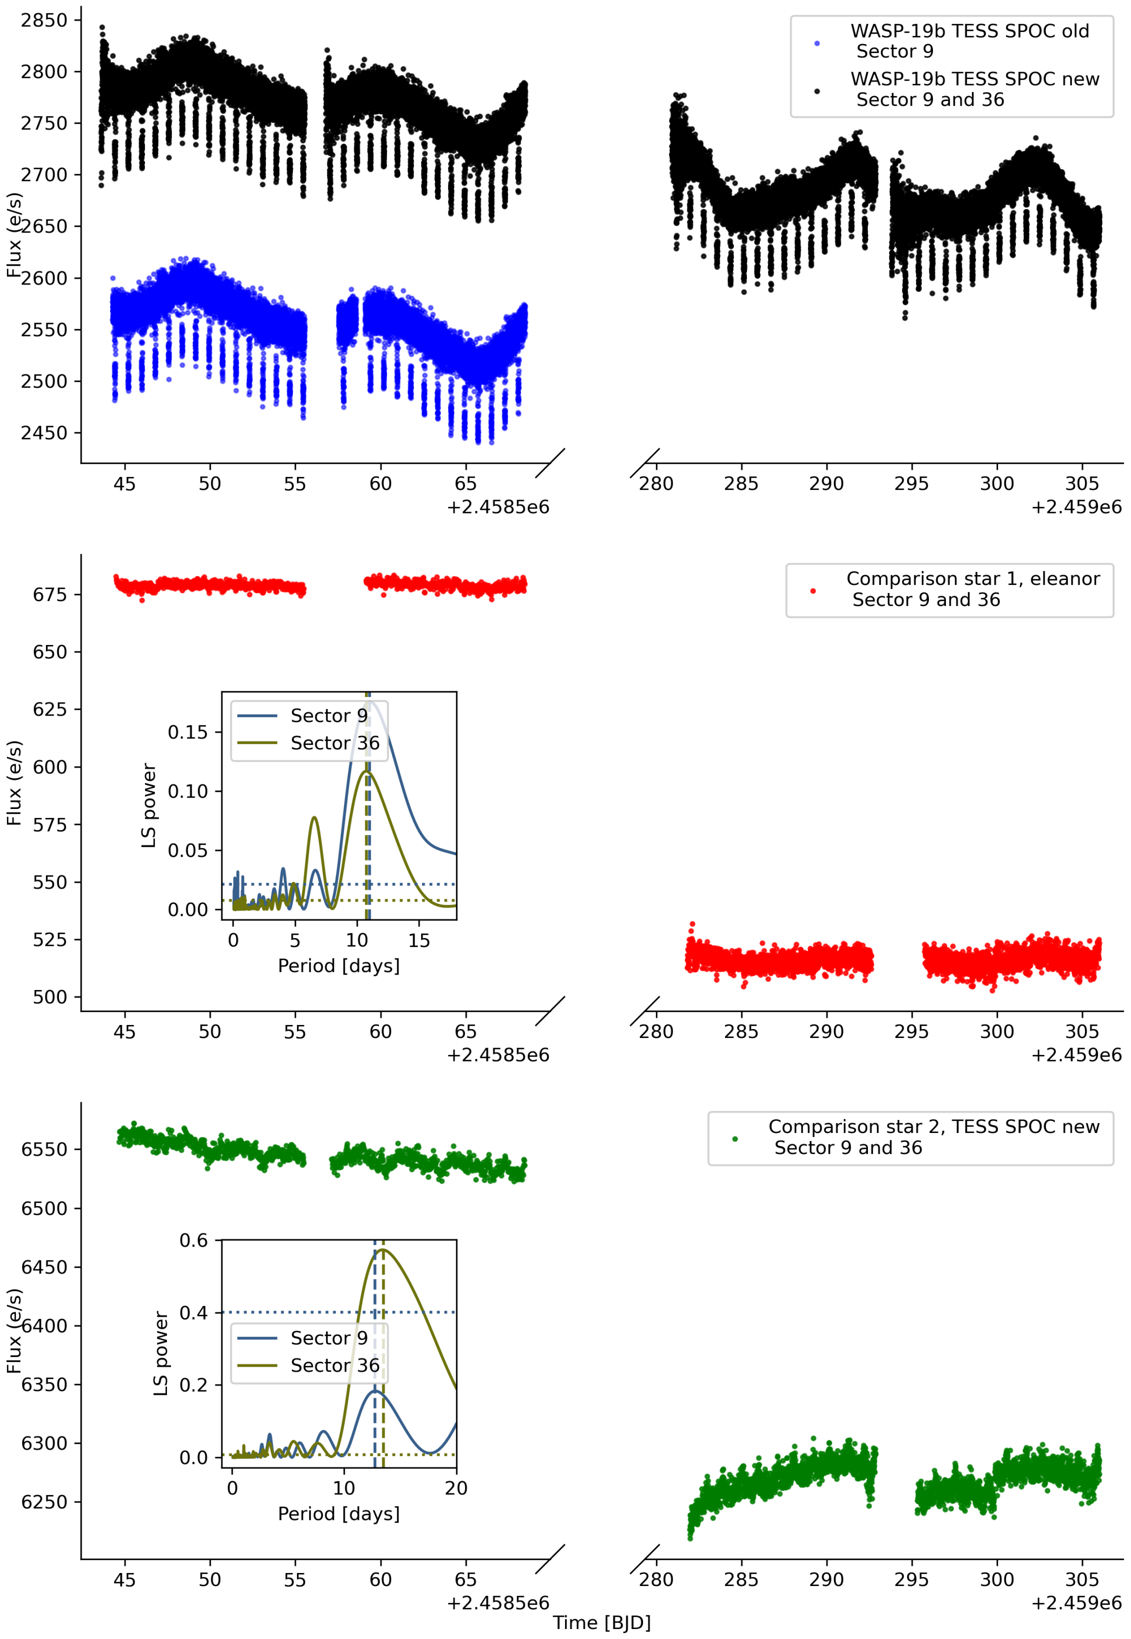


Figure 11: TESS sector 9 and 36 (left and right parts respectively of top, middle, and bottom panels) light curves of WASP-19, comparison star 1, and 2. Both sector 9 and 36 data for for WASP-19 were analysed by an update to the TESS SPOC pipeline plotted in black in the top panel along with the sector 9 data from the older version of TESS SPOC pipeline plotted in blue. Middle and bottom panels show the Sector 9 and 36 light curves and their Lomb Scargle (LS) periodograms (horizontal dashed lines marking the 10 % false alarm probability levels and vertical lines marking the peak of the periodogram) for comparison star 1 and 2 using `eleanor` and the new version of TESS SPOC pipeline respectively. The comparison star 1 LS periodogram peaks at 11 days and 10.74 days for sector 9 and 36 respectively. The comparison star 2 LS periodogram peaks at 12.72 days and 13.48 days for sector 9 and 36 respectively. Further details of the analysis of TESS data are described in Appendix A1.

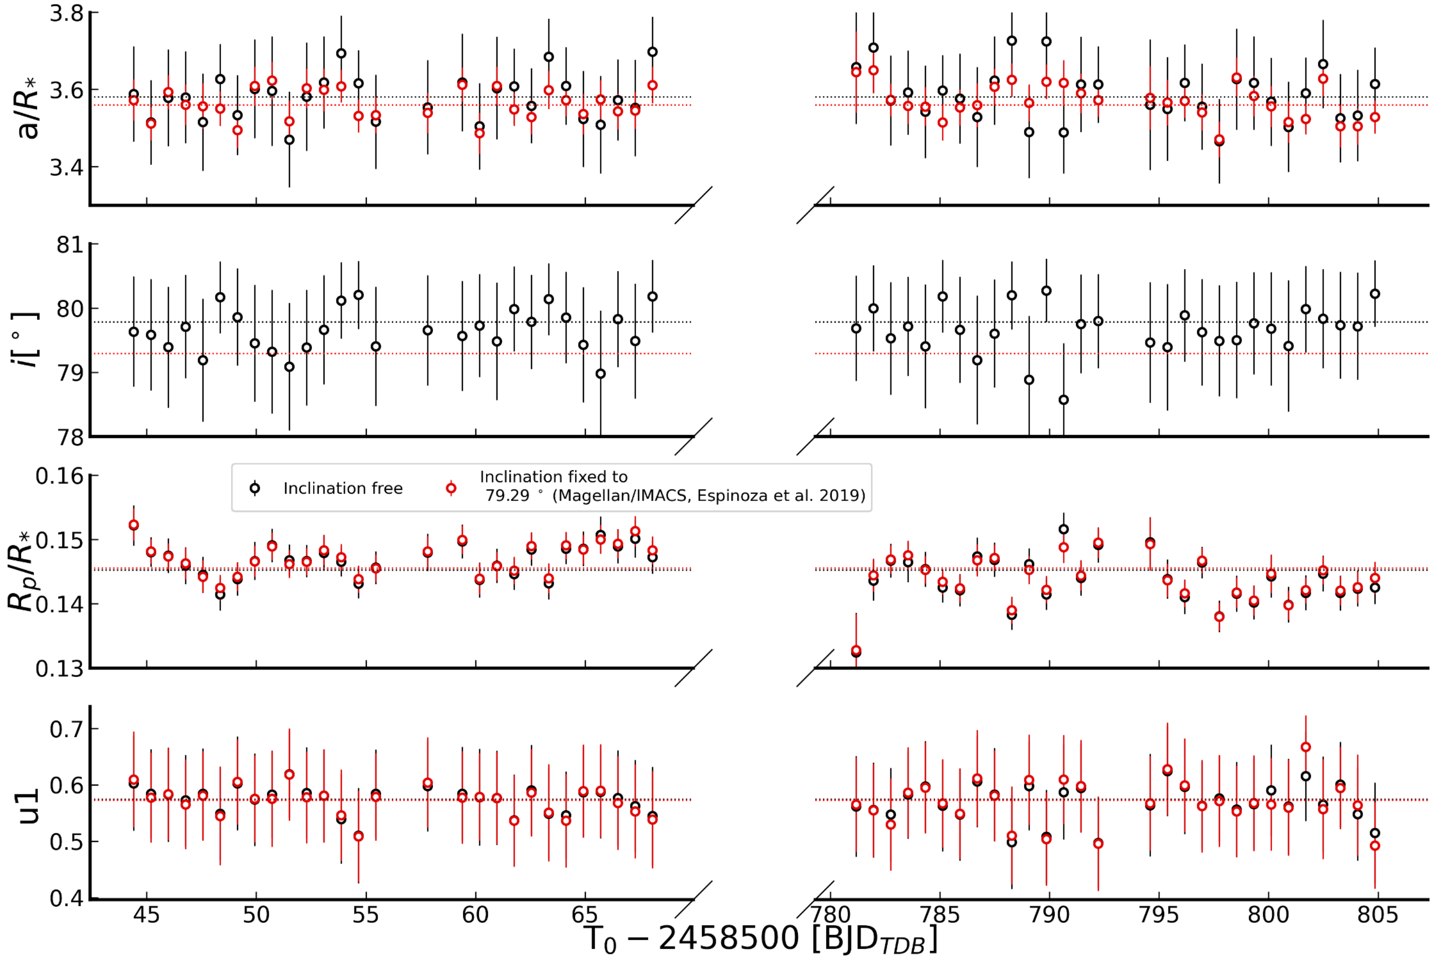


Figure 12: Best fit transit parameters of WASP-19 from the light curves obtained in the TESS sector 9 and 36 (left and right parts respectively of top, middle, and bottom panels). The black points for all the parameters are the best fit values for each transit obtained by fitting for all parameters including inclination, with the horizontal dashed black lines showing the weighted average value across all 58 transits. The red points are the best fit values for a/R$_*$, $R_p/R_*$, and u$_1$ when fixing the inclination to the value reported by the Magellan/IMACS observations, with the red dashed line showing their respective weighted average values. The horizontal red dashed line in the inclination panel marks the inclination measured by Magellan/IMACS observations.

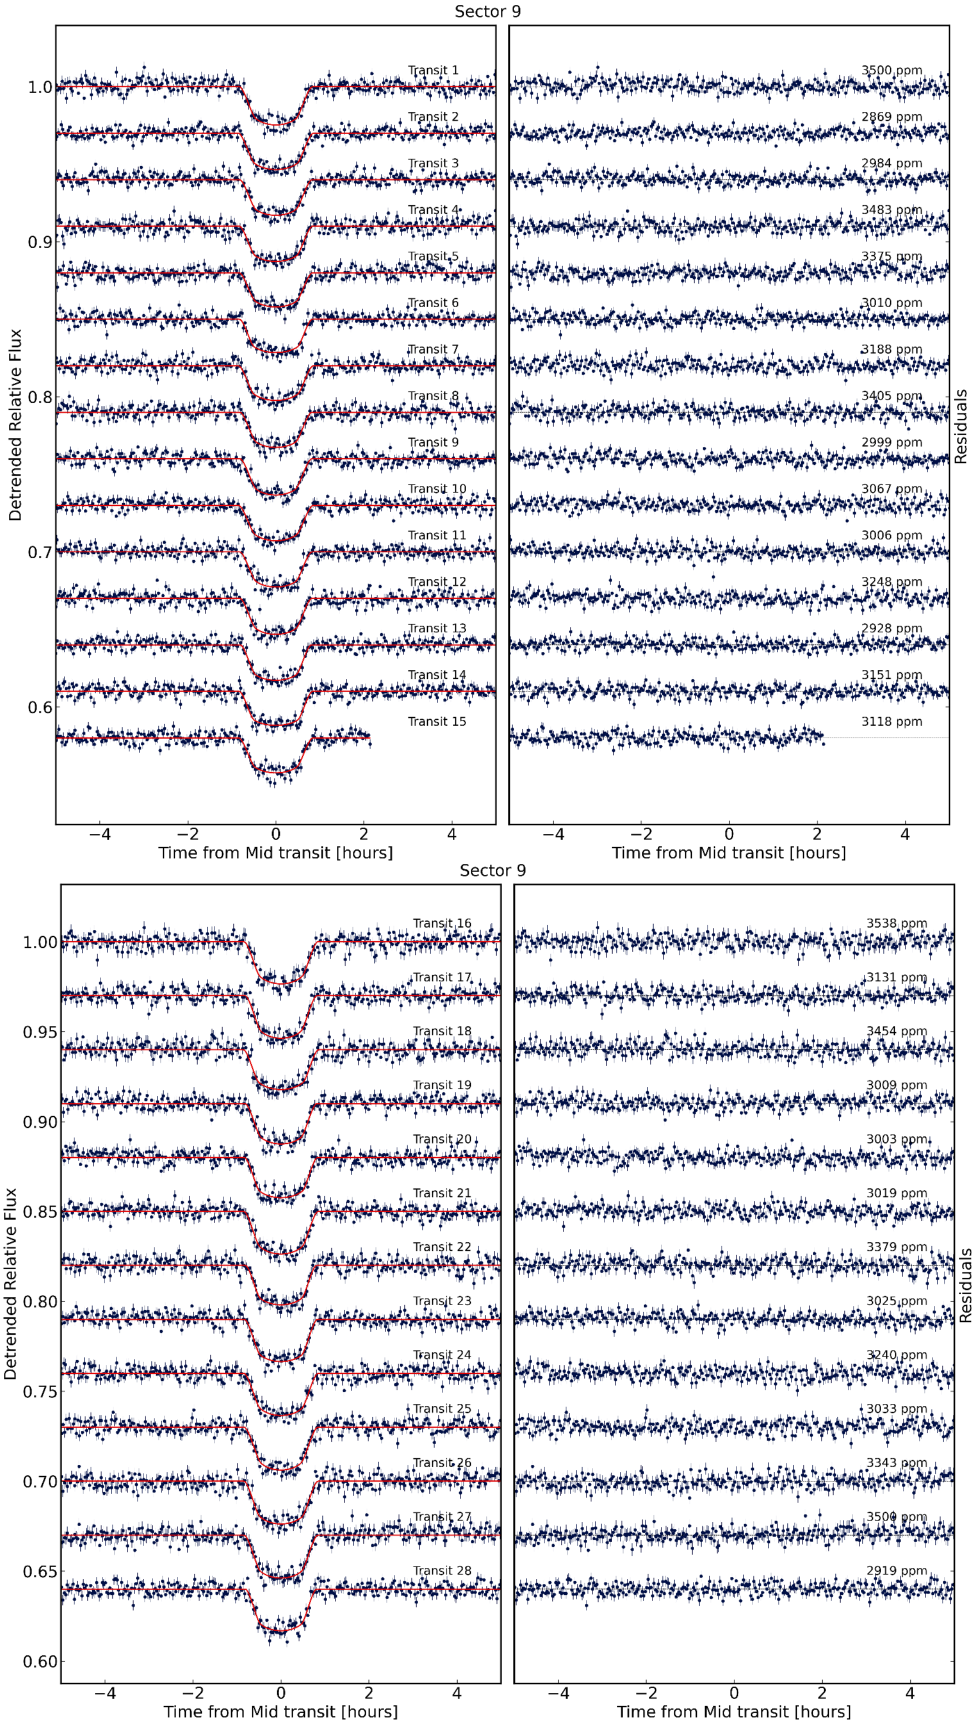


Figure 13: Transit light curves for WASP-19b observed by TESS with their best fit transit model overplotted in red. The data are detrended SAP light curves secured in sector 9 and released on MAST through the latest TESS SPOC pipeline. The top two panels are the light curves from the first half of sector 9 and the bottom two panels are from the second half after the mid-sector change of TESS orbit. The right panels both top and bottom shows the residuals to the best fits for each transit along with the RMS of the residuals.

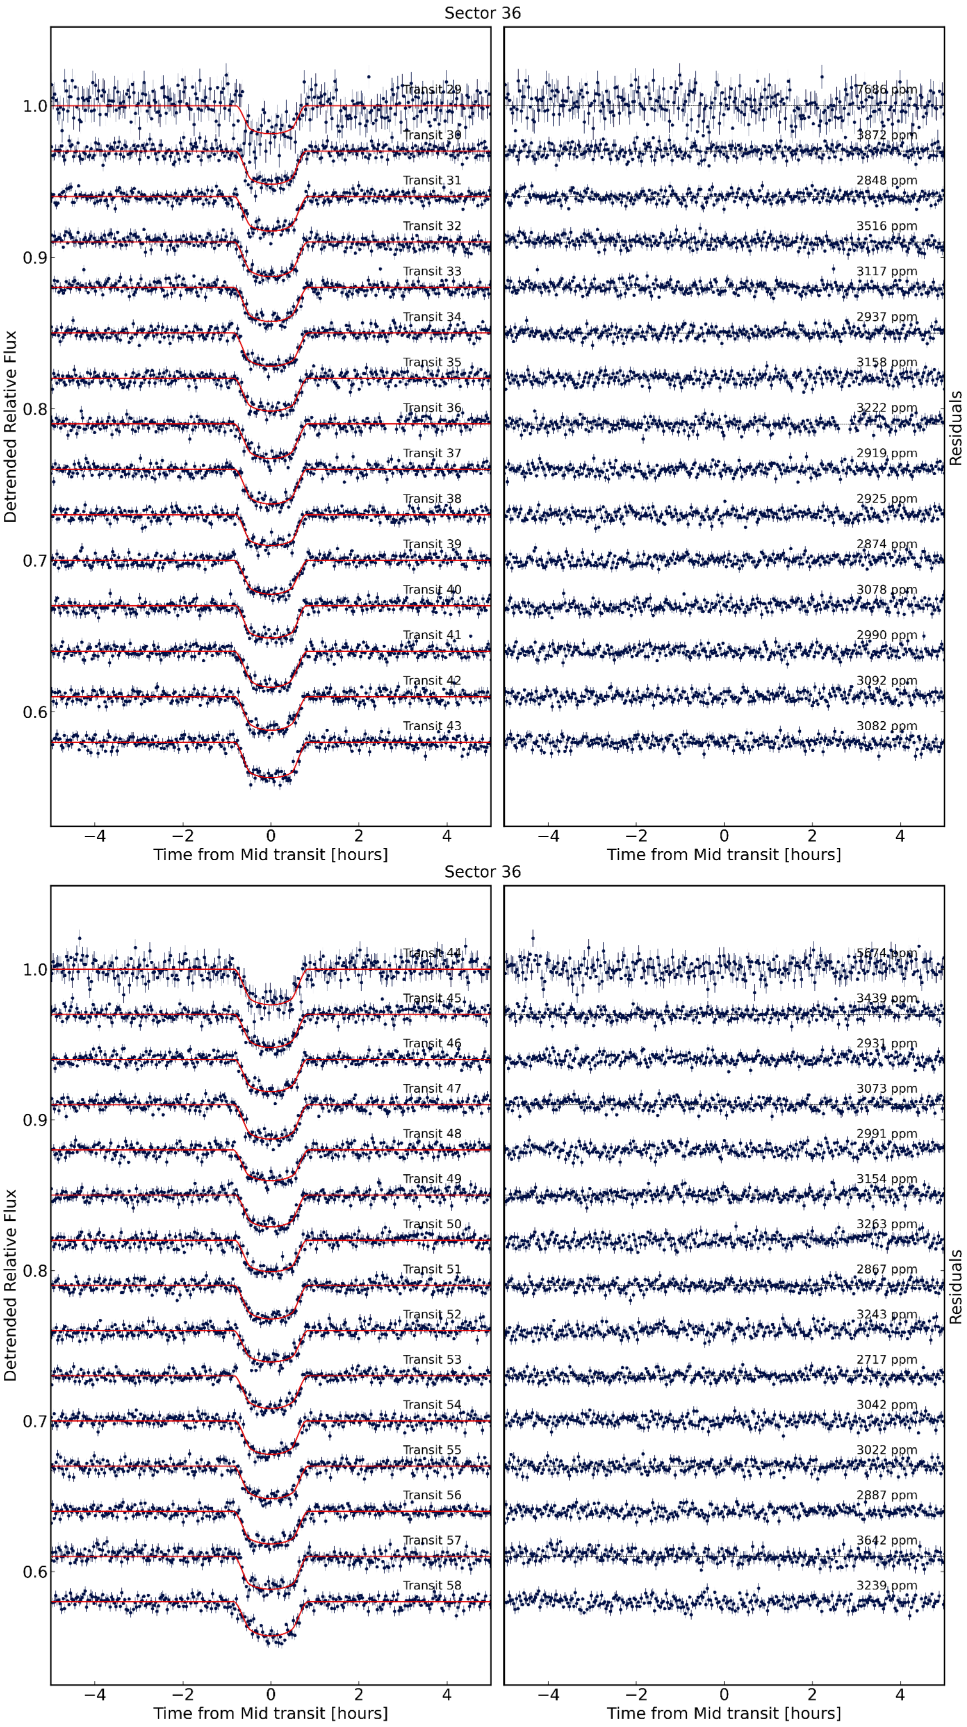


Figure 14: Same as Figure 13 but for sector 36.
